# Supplementary material for: Behind the Scenes: An Exploration of Trigger Biases Problem in Few-Shot Event Classification
Source: arXiv:2108.12844 source file (2021-08-29)
Supplement: Supplementary file 1 [file appendix.tex]

\section{Detailed Dataset Division}
\label{sec:dataset-division}

In our paper, we conduct experiments mainly on MAVEN\footnote{\url{https://github.com/THU-KEG/MAVEN-dataset}} and FewEvent\footnote{\url{https://github.com/231sm/Low_Resource_KBP}} dataset.
There is no unified criterion for dataset division in Few-Shot Event Detection studies.
Therefore, to facilitate the potential follow-up studies, we also illustrate the specific dataset division in our paper.
Figure~\ref{fig:my-label-maven} shows the dataset divison for MAVEN, and Figure~\ref{fig:my-label-fewevent} shows the dataset division for FewEvent.

\begin{figure*}[h]
    \centering
    \includegraphics[width=0.6\linewidth]{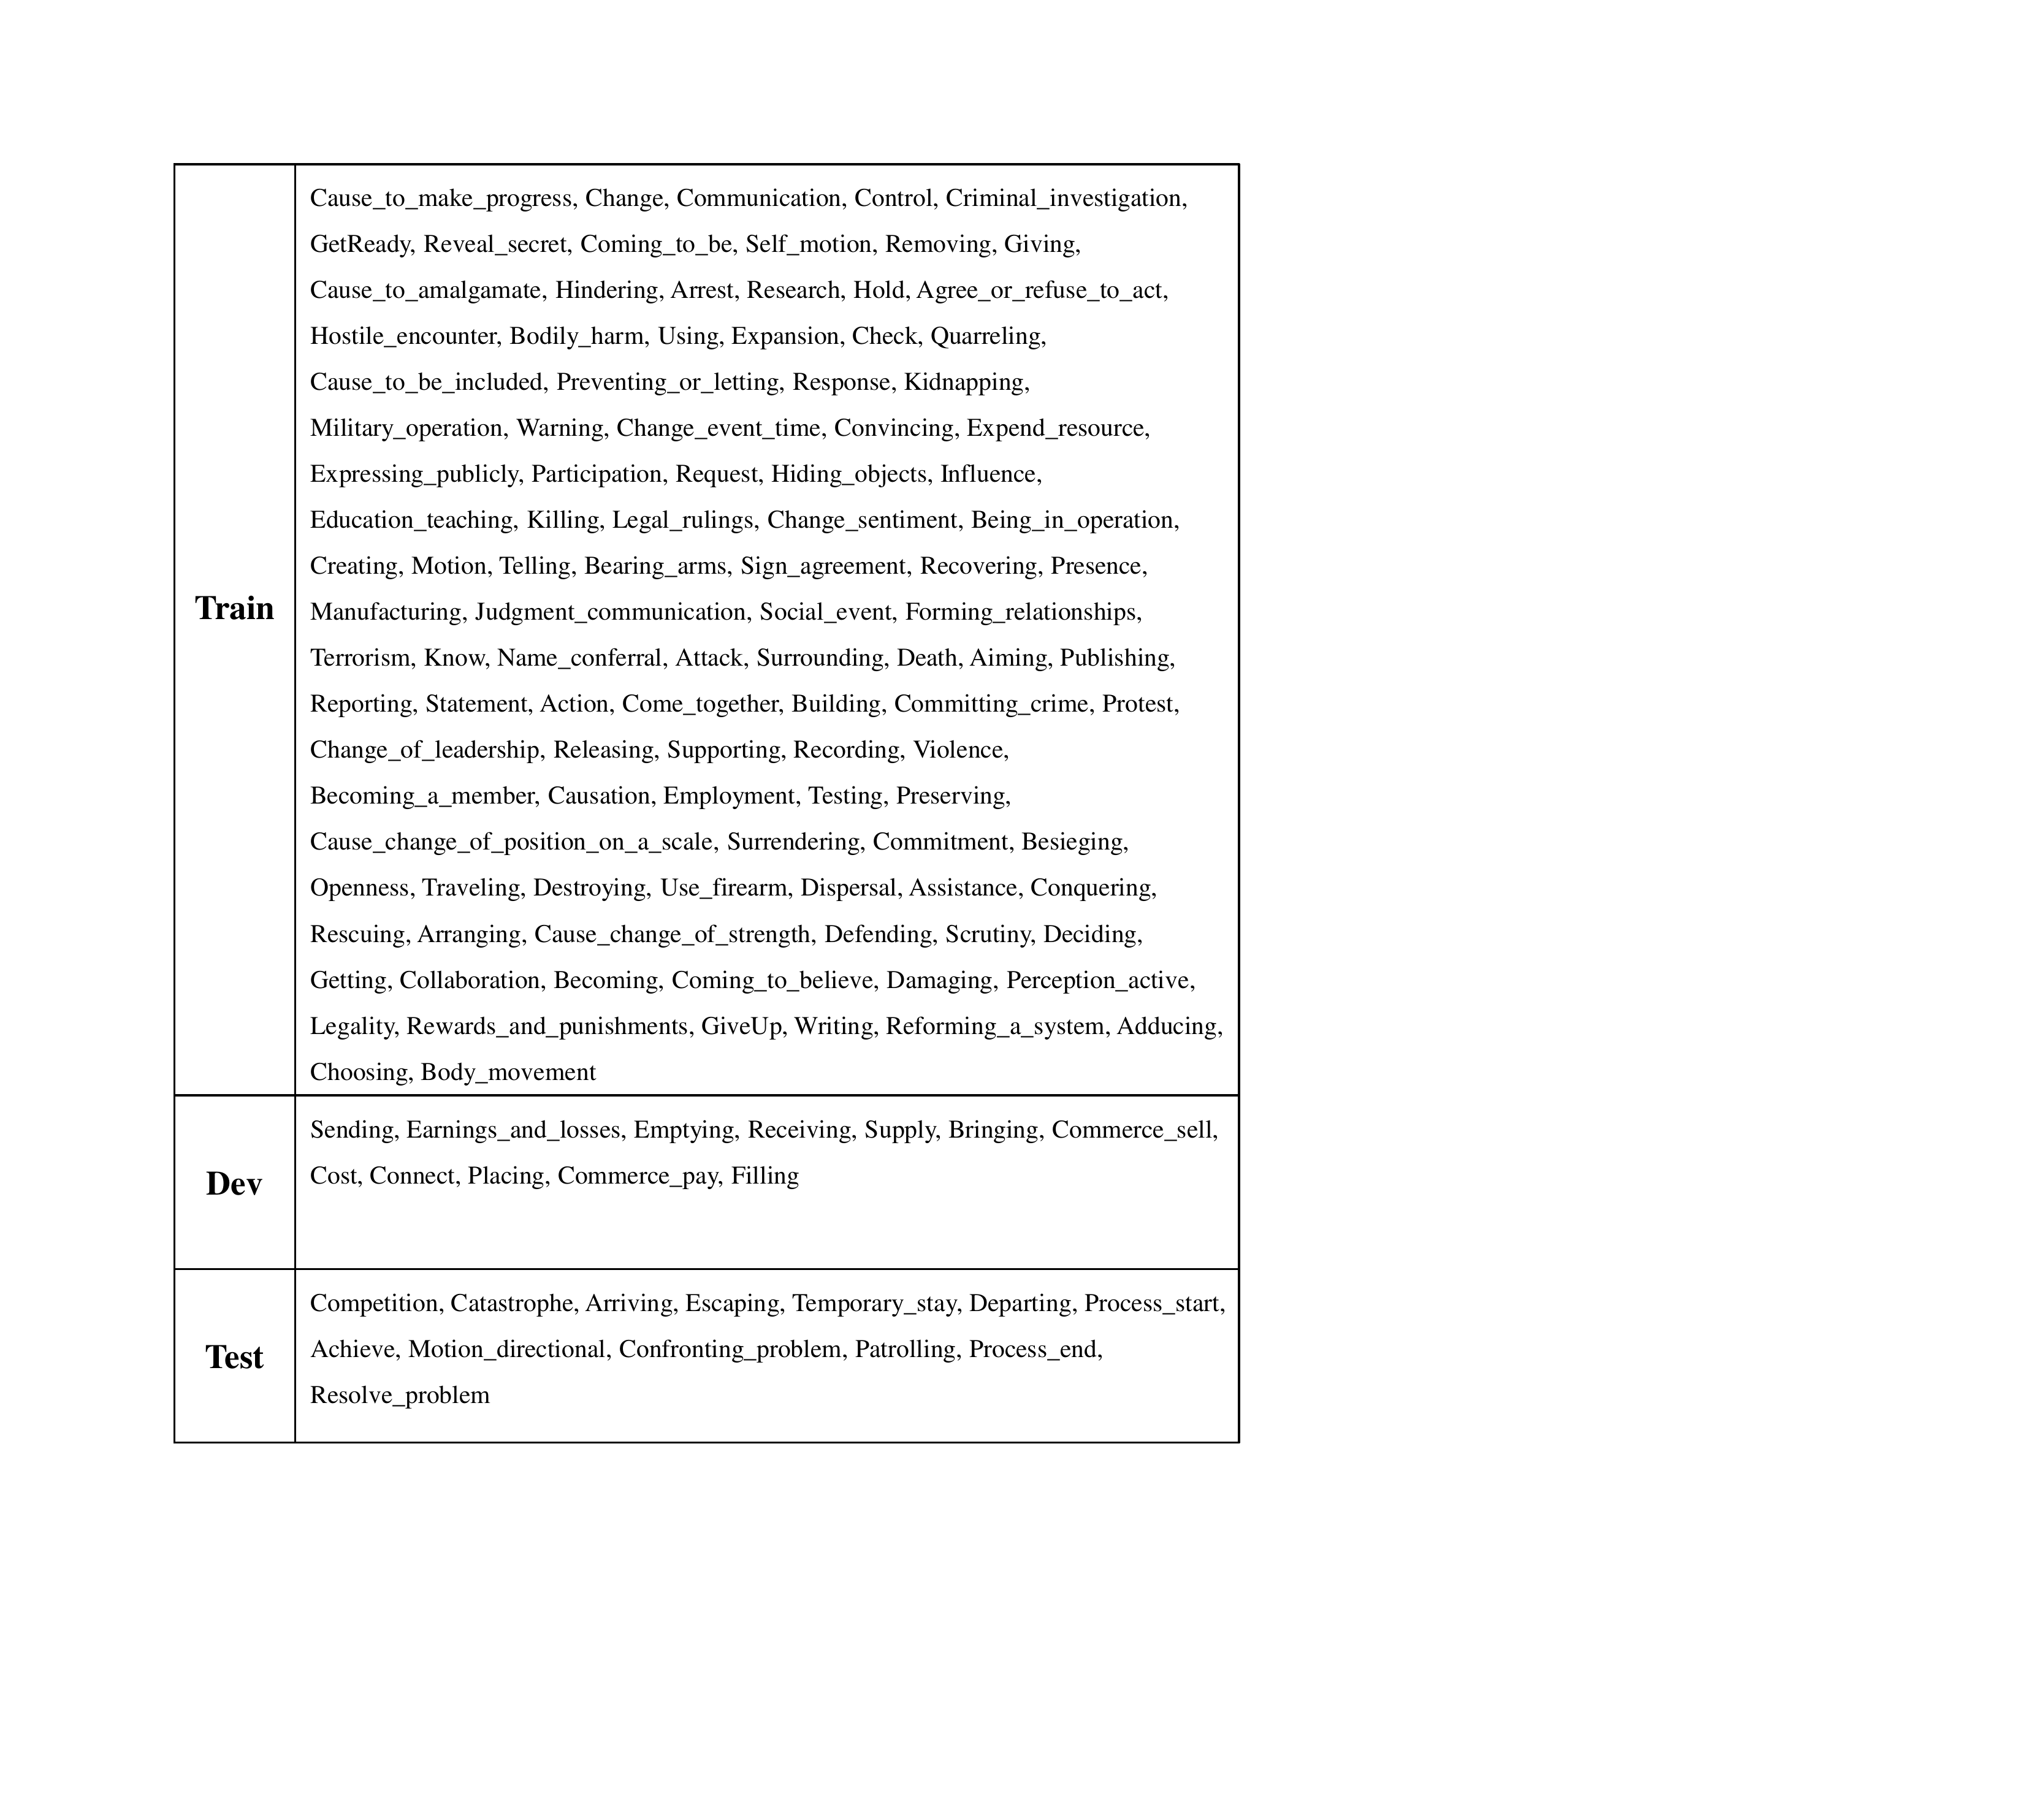}
    \caption{Dataset Division for MAVEN. The table illustrates specific event types in train/dev/test set.}
    \label{fig:my-label-maven}
\end{figure*}
\begin{figure*}[h]
    \centering
    \includegraphics[width=0.6\linewidth]{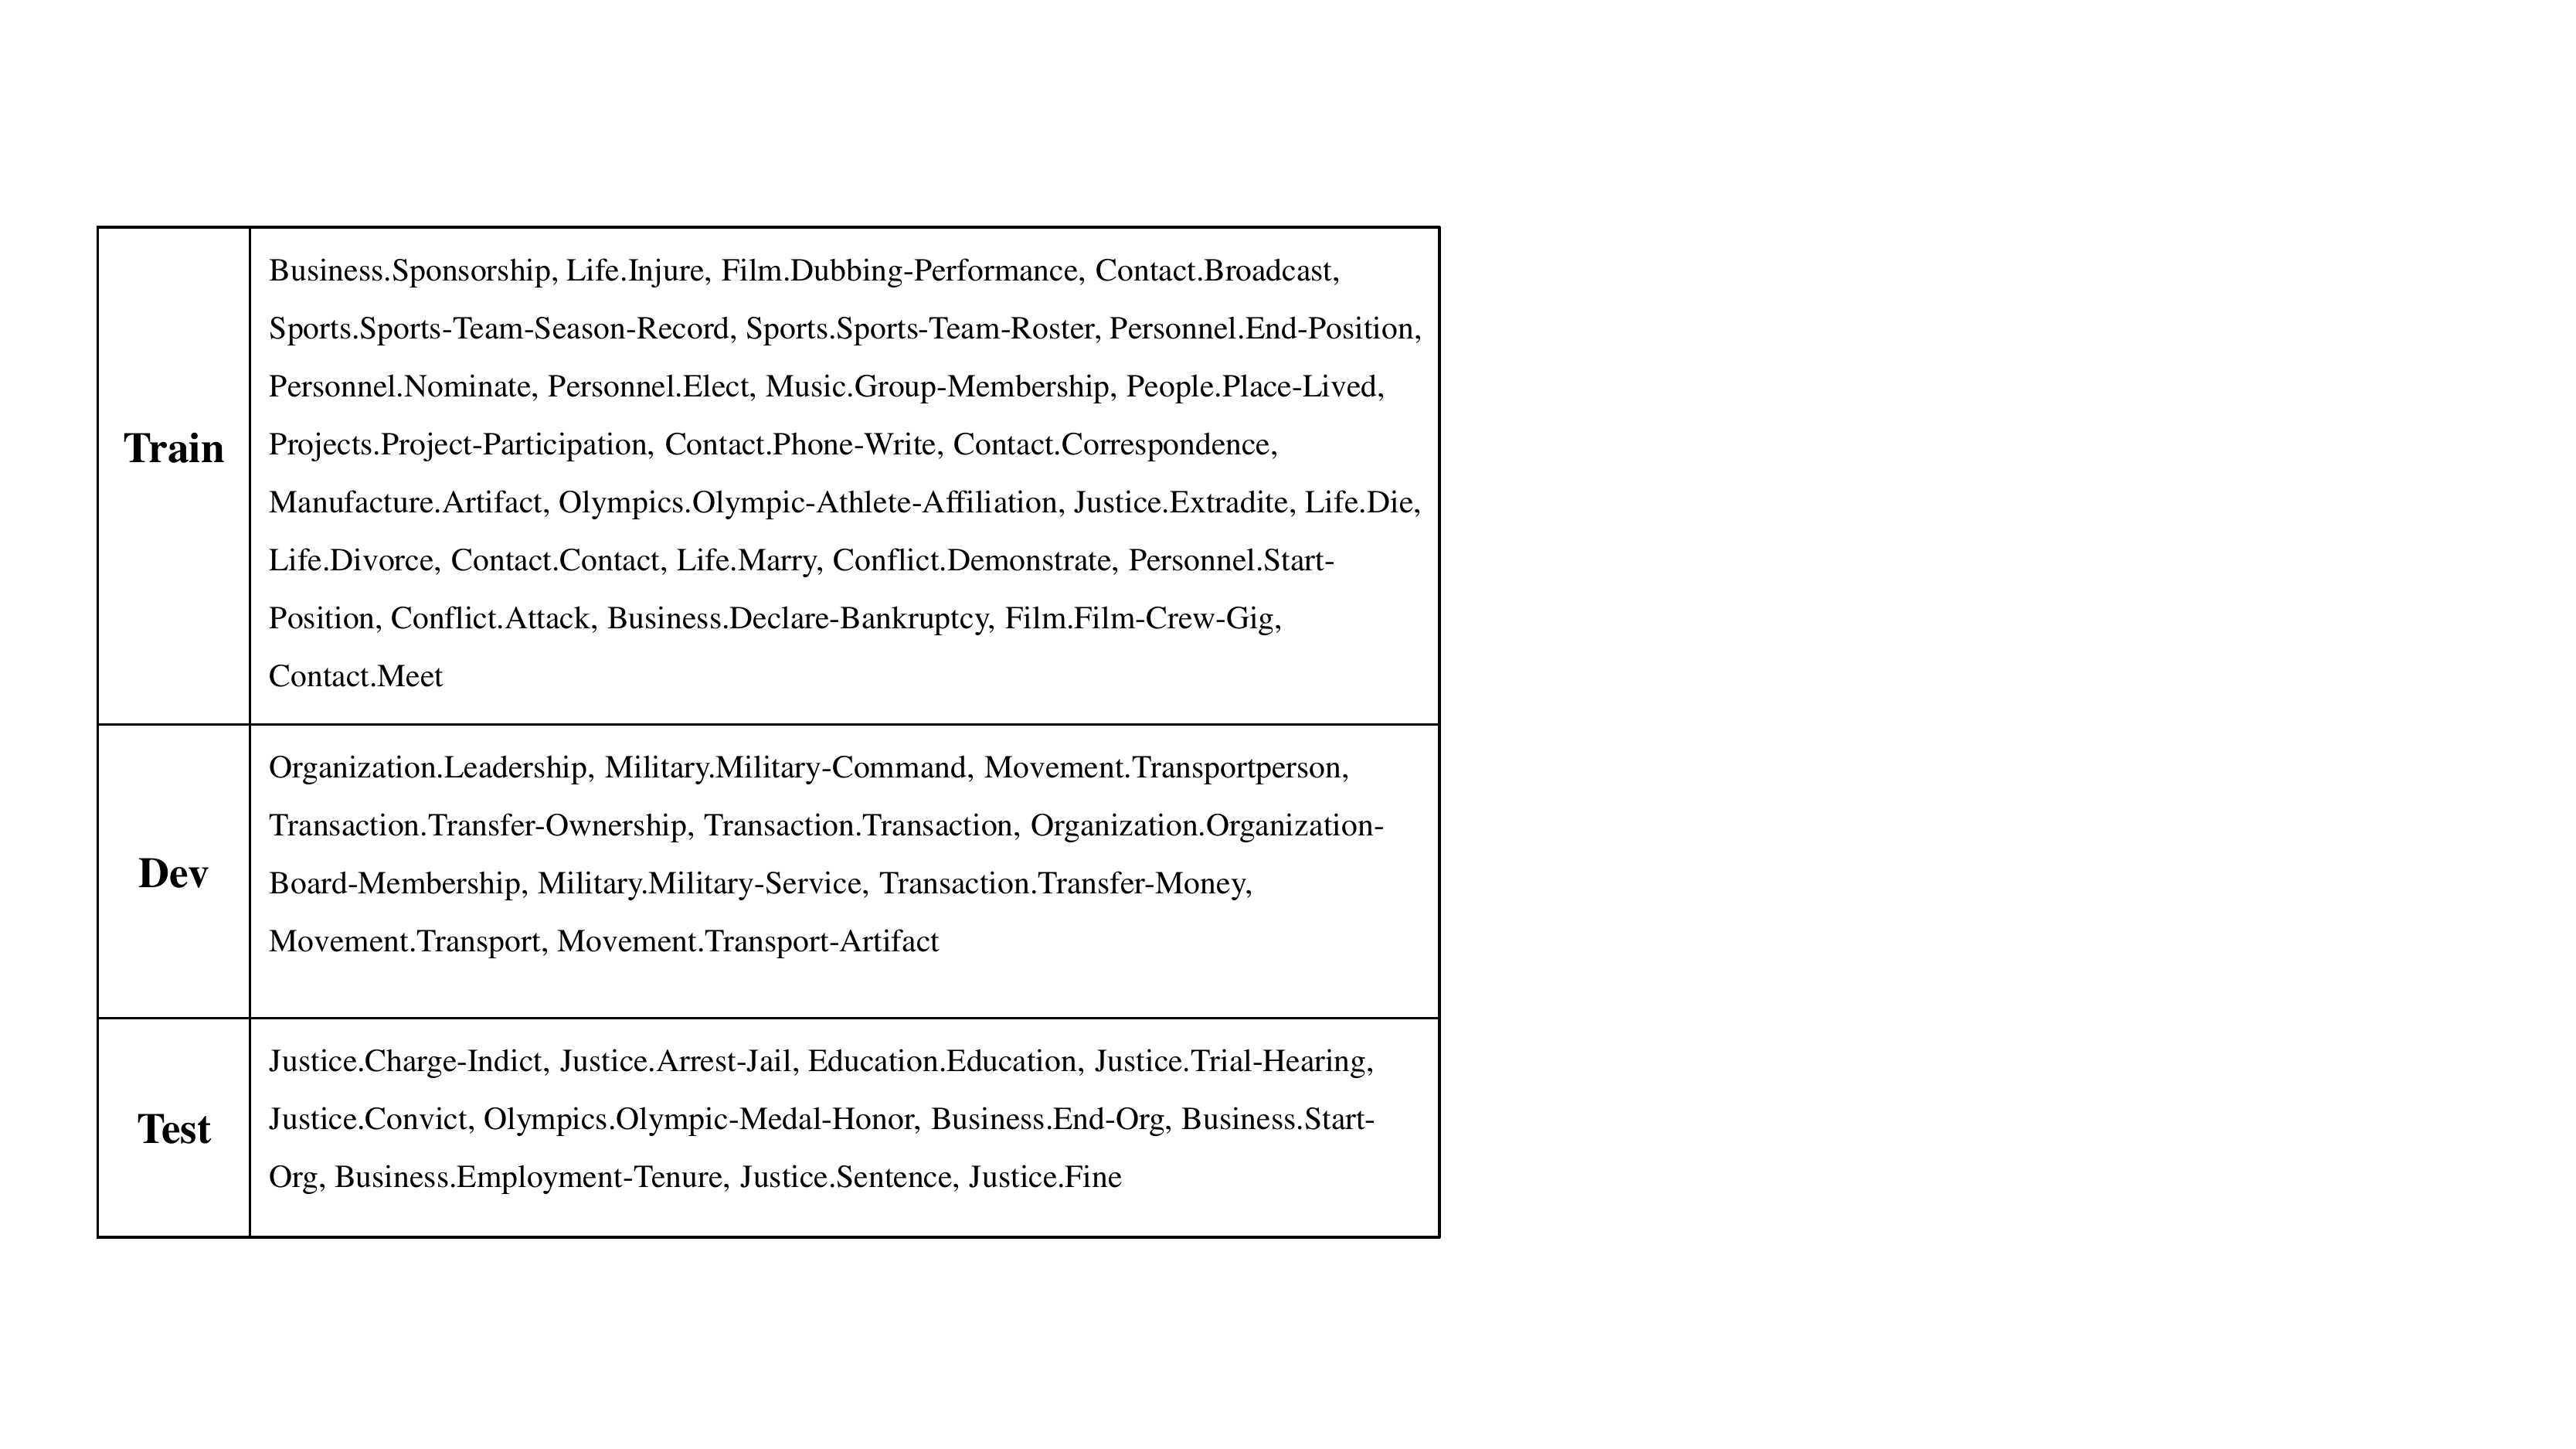}
    \caption{Dataset Division for FewEvent. The table illustrates specific event types in train/dev/test set.}
    \label{fig:my-label-fewevent}
\end{figure*}
